# Supplementary material for: Incorporating Participants' Welfare into Sequential Multiple Assignment Randomized Trials
Source: arXiv:2210.16255 source file (2023-09-19)
Supplement: Supplementary file 1 [file Supp.pdf]

# Supporting Information for "SMART-EXAM: Incorporating Participants' Welfare into Sequential Multiple Assignment Randomized Trials"

Xinru Wang, Nina Deliu, Yusuke Narita, and Bibhas Chakraborty

October 29, 2022

## Web Appendix A: A two-stage SMART-EXAM with two treatment options at each stage, where the randomization probabilities are individualized at both stages.

Define the stage-2 Q-function for those who don't respond to the initial treatment as

$$Q_2(\boldsymbol{H}_{2i}, A_{2i}; \boldsymbol{\gamma}_2, \boldsymbol{\alpha}_2) = \boldsymbol{\gamma}_2^T \boldsymbol{H}_{20i} + \boldsymbol{\alpha}_2^T \boldsymbol{H}_{21i} A_{2i}, \tag{1}$$

where $\boldsymbol{\gamma}_2$ and $\boldsymbol{\alpha}_2$ are estimated through OLS:

$$(\hat{\boldsymbol{\gamma}}_2, \hat{\boldsymbol{\alpha}}_2) = \underset{\boldsymbol{\gamma}_2, \boldsymbol{\alpha}_2}{\arg\min} \sum_{i=1} (Y_i - Q_2(\boldsymbol{H}_{2i}, A_{2i}; \boldsymbol{\gamma}_2, \boldsymbol{\alpha}_2))^2. \tag{2}$$

Define stage-1 Q-functions as

$$Q_1(\boldsymbol{H}_{1i}, A_{1i}; \boldsymbol{\gamma}_1, \boldsymbol{\alpha}_1) = \boldsymbol{\gamma}_1^T \boldsymbol{H}_{10i} + \boldsymbol{\alpha}_1^T \boldsymbol{H}_{11i} A_{1i}, \tag{3}$$

and $\boldsymbol{\gamma}_1, \boldsymbol{\alpha}_1$ can be estimated by:

$$(\hat{\boldsymbol{\gamma}}_1, \hat{\boldsymbol{\alpha}}_1) = \underset{\boldsymbol{\gamma}_1, \boldsymbol{\alpha}_1}{\arg\min} \sum_{i=1}^{N} (\tilde{Y}_i - Q_1(\boldsymbol{H}_{1i}, A_{1i}; \boldsymbol{\gamma}_1, \boldsymbol{\alpha}_1))^2, \tag{4}$$

where $\tilde{Y}_i = \max_{a_2 \in \{-1,1\}} Q_2(\boldsymbol{H}_2, a_2; \hat{\boldsymbol{\gamma}}_2, \hat{\boldsymbol{\alpha}}_2)$ is the stage-1 pseudo-outcome for the $i$-th participant.

Upon enrollment, the researchers collect the baseline covariates $\boldsymbol{O}_1$, such as age, gender, and race. The parameters $\boldsymbol{\gamma}_1$ and $\boldsymbol{\alpha}_1$ in Formula (3) are estimated using Formula (4) based on the pilot/previous SMART or observational studies, which are then used in combination with the collected patient history data $\boldsymbol{O}_1$ to predict the stage-1 individualized treatment effect $\hat{\zeta}_{1,i} = 2\hat{\boldsymbol{\alpha}}_1^T \boldsymbol{H}_{11i}$. With the predicted treatment effects and elicited preference data, the procedure of generating randomization probabilities for stage-1 treatments is the same as the procedure described in Section 4.2 of the main paper, through which the participants are randomized to available stage-1 treatment options.

# Web Appendix B: Algorithm for the SMART-EXAM

**Algorithm 1**

**Input:** $C_{a_2|a_1}$: the capacity for stage-2 treatment $a_2$ for non-responders to initial treatment $a_1$; $\Lambda_i$: the preference indicator for the $i$-th participant; $m$: the budget for "buying" randomization probabilities for stage-2 treatment $A_2 = 1$; $\hat{\zeta}_i$: the predicted effect of receiving treatment $A_2 = 1$ instead of $A_2 = -1$ on the outcome for the $i$-th participant; $\eta$: the coefficient of treatment effects in the price function; ClearThreshold: the threshold for the market clearing error; IterationThreshold: the threshold for iteration times

**Output:** $p_{2,a_2,i}$: the individualized randomization probabilities for the non-responders; $\beta^*$: the intercept in the price function

**function** INITBETA ▷ Set the initial value of $\beta$
  $\beta \longleftarrow (-\max_i |\hat{\zeta}_i|, 0)$
  **return** $\beta$
**end function**
**function** PRICE($\eta$, $\beta$, $\zeta_i$) ▷ Get the price of unit randomization probability of treatment $A_2 = 1$
  **for** $i \in 1, \ldots, N_{a_1}$ **do**
    $\Psi_i = \eta\zeta_i + \beta$
  **end for**
  **return** $\Psi_i$
**end function**
**function** DEMAND($\Psi_i$,$m = 1$, $\Lambda_i$) ▷ Solve the utility maximization function subject to the budget constraint
  **for** $i \in 1, \ldots, N_{a_1}$ **do**
    $p_{2,1,i} \longleftarrow \arg\max_{p_{2,1,i} \in \mathcal{P}} u_i \quad s.t.\ p_{2,1,i}\ \Psi_i \leq m$ ▷ $u_i = p_{2,1,i}\Lambda_i + (1 - p_{2,1,i})(1 - \Lambda_i)$
  **end for**
**end function**
**function** EXCESSDEMAND($\Psi_i$) ▷ Get the excess demand for stage-2 treatment
  **for** $a_2 \in \{1, -1\}$ **do**
    $d_{a_2} \longleftarrow \sum_i^{N_{a_1}} p_{2,a_2,i} - C_{a_2|a_1}$
  **end for**
  **return** $d_{a_2}$
**end function**
**function** CLEARERROR($d_{a_2}$). ▷ Get the market clear error
  **if** $d_{a_2} < 0$ for all $a_2$ **then**
    **return** 0
  **else**
    error $\longleftarrow \sqrt{\sum_{a_2} d_{a_2}^2} / \{\sum_{a_2} C_{a_2|a_1}\}$
  **end if**
  **return** error
**end function**

**Algorithm 1** (continued)

```
function BETANEW(β, d)                                ▷ Adjust β to set new prices
    for i ∈ 1, ..., N_{a_1} do
        β^{new} ⟵ β + d × m/50
    end for
     return β^{new}
end function
function MAIN
    for a_1 ∈ {−1, 1} do
        β ⟵ INITBETA()
        for i ∈ 1, ..., N_{a_1} do
            Ψ_i ⟵ PRICE(η, β, ζ_i)
            p_{2,1,i} ⟵ DEMAND(Ψ_i, m, Λ_i)
        end for
        d_{a_2} ⟵ EXCESSDEMAND(Ψ_i)
        error ⟵ CLEARERROR(d_{a_2})
        error^{min} ⟵ error
        ClearThreshold ⟵ 0.02
        IterationThreshold ⟵ 500
        Iteration ⟵ 0
        while True do
            if Iteration > IterationThreshold then
                β ⟵ INITBETA()
                Iteration ⟵ 0
            else
                β ⟵ BETANEW(β, d)
                for i ∈ 1, ..., N_{a_1} do
                    Ψ_i ⟵ PRICE(η, β, ζ_i)
                    p_{2,1,i} ⟵ DEMAND(Ψ_i, m, Λ_i)
                end for
                d_{a_2} ⟵ EXCESSDEMAND(Ψ_i)
                error ⟵ CLEARERROR(d_{a_2})
            end if
            if error < error_{min} then
                error_{min} ⟵ error
                β* ⟵ β
                p*_{2,1,i} ⟵ p_{2,1,i}
            end if
            if error_{min} < ClearThreshold then
                Break
            end if
            Iteration += 1
        end while
    end for
    return p*_{2,1,i}, β*
end function
```

# Web Appendix C: Proof of Theorems

## Theorem 1

Assume there is a SMART-EXAM design with capacity $C_{a_2|a_1}$. When the patients' preferences and predicted treatment effects are not of concern, this SMART-EXAM can be reduced to the regular SMART design with non-individualized assignment probabilities $p^0_{2,a_2} = \frac{C_{a_2|a_1}}{N_{a_1}}$, by setting $\Lambda_i = \Lambda_j = 1$ and $\hat{\zeta}_i = \hat{\zeta}_j$ for all $i$ and $j$ ($j \neq i$) among non-responders to $a_1$.

*Proof.* Suppose on the contrary that there are some $\tilde{p}_{2,1,i}$ such that $\tilde{p}_{2,1,i} \neq p^0_{2,1}$. Given the condition that $\hat{\zeta}_i = \hat{\zeta}_j$ for all $i$ and $j$ ($j \neq i$), the treatment prices for all participants are the same. With $\Lambda_i = \Lambda_j = 1$, the utility function for each participant is the same, so $\tilde{p}_{2,1,i} = \tilde{p}_{2,1,j} \neq p^0_{2,1}$.

If $\tilde{p}_{2,1,i} = \tilde{p}_{2,1,j} > p^0_{2,1} = \frac{C_{1|a_1}}{N_{a_1}}$, then $\sum_i^{N_{a_1}} \tilde{p}_{2,1,i} > \frac{N_{a_1} C_{1|a_1}}{N_{a_1}} = C_{1|a_1}$, which is a contradiction to the capacity constraint $\sum_i^{N_{a_1}} p_{2,1,i} = C_{1|a_1}$.

If $\tilde{p}_{2,1,i} = \tilde{p}_{2,1,j} < p^0_{2,1} = \frac{C_{1|a_1}}{N_{a_1}}$, then $\tilde{p}_{2,-1,i} = \tilde{p}_{2,-1,j} > p^0_{2,-1} = \frac{C_{-1|a_1}}{N_{a_1}}$. We can get $\sum_i^{N_{a_1}} \tilde{p}_{2,-1,i} > \frac{N_{a_1} C_{-1|a_1}}{N_{a_1}} = C_{-1|a_1}$, which is a contradiction to the capacity constraint $\sum_i^{N_{a_1}} p_{2,-1,i} = C_{-1|a_1}$.

Given above, we can get $\tilde{p}_{2,1,i} = p^0_{2,1}$ for all non-responders to the initial treatment $a_1$ when setting $\Lambda_i = \Lambda_j = 1$ and $\hat{\zeta}_i = \hat{\zeta}_j$ for all $i$ and $j$ ($j \neq i$), in which SMART-EXAM is the same as the typical SMART with non-individualized stage-2 randomization probabilities $p^0_{2,a_2} = \frac{C_{a_2|a_1}}{N_{a_1}}$. □

## Theorem 2

To facilitate the proof of the consistent estimator and its asymptotic normality property, we introduce three assumptions under Neyman-Rubin causal framework:

- Sequential exchangeability assumption (SEA):

  Under SEA, the treatment allocation at each stage is independent of the potential outcomes conditional on the historical data. In a two-stage SMART-EXAM, $R^{A_1} \perp A_1$, $Y^{\boldsymbol{d}_j} \perp A_1$, and $Y^{\boldsymbol{d}_j} \perp A_2 | A_1, R^{A_1}, G^{A_1}$.

- Consistency assumption (CA):

  The potential outcome under the observed treatment is the outcome that is actually observed for an individual. In a two-stage SMART-EXAM, $Y^{\boldsymbol{d}_j} = Y$ if the patient is randomized to DTR $\boldsymbol{d}_j = (a_1, a_2)$; $R^{a_1} = R$ if $A_1 = a_1$.

- Positivity assumption (PA):

  If the probability of the history data is positive, the randomization probabilities for all the treatment options should be positive.

### Consistency

*Proof.* Under the Consistency assumption (CA), the Sequential exchangeability assumption (SEA),

and the Positivity assumption (PA), we can get:

$$
\begin{aligned}
\mu_{\boldsymbol{d}_j} &= E[Y_i^{\boldsymbol{d}_j}] = E[E[Y_i^{\boldsymbol{d}_j}|R_i^{a_1}]] \\
&= \Pr(R_i^{a_1}=1)E[Y_i^{\boldsymbol{d}_j}|R_i^{a_1}=1] + \Pr(R_i^{a_1}=0)E[Y_i^{\boldsymbol{d}_j}|R_i^{a_1}=0] \\
&= \Pr(R_i^{a_1}=1|A_{1i}=a_1)E[Y_i^{\boldsymbol{d}_j}|A_{1i}=a_1, R_i^{a_1}=1, A_{2i}=a_2] + \Pr(R_i^{a_1}=0)E[Y_i^{\boldsymbol{d}_j}|R_i^{a_1}=0] \\
&\text{(According to SEA)} \\
&= \Pr(R_i=1|A_{1i}=a_1)E[Y_i|A_{1i}=a_1, R_i=1, A_{2i}=a_2] + \Pr(R_i^{a_1}=0)E[Y_i^{\boldsymbol{d}_j}|R_i^{a_1}=0] \\
&\text{(According to CA)} \\
&= \pi_{a_1}\mu_{s(a_1,a_1)} + \Pr(R_i^{a_1}=0)E[E[Y_i^{\boldsymbol{d}_j}|R_i^{a_1}=0, G_i^{a_1}]|R_i^{a_1}=0] \\
&= \pi_{a_1}\mu_{s(a_1,a_1)} + \Pr(R_i^{a_1}=0)\sum_g \Pr(G_i^{a_1}=g|R_i^{a_1}=0)E[Y_i^{\boldsymbol{d}_j}|R_i^{a_1}=0, G_i^{a_1}=g] \\
&= \pi_{a_1}\mu_{s(a_1,a_1)} + \sum_g \Pr(R_i^{a_1}=0, G_i^{a_1}=g)E[Y_i^{\boldsymbol{d}_j}|R_i^{a_1}=0, G_i^{a_1}=g] \\
&= \pi_{a_1}\mu_{s(a_1,a_1)} + \sum_g \Pr(R_i^{a_1}=0, G_i^{a_1}=g|A_{1i}=a_1)E[Y_i^{\boldsymbol{d}_j}|A_{1i}=a_1, R_i^{a_1}=0, G_i^{a_1}=g, A_{2i}=a_2] \\
&\text{(According to SEA)} \\
&= \pi_{a_1}\mu_{s(a_1,a_1)} + \sum_g \Pr(R_i=0, G_i=g|A_{1i}=a_1)E[Y_i|A_{1i}=a_1, R_i=0, G_i=g, A_{2i}=a_2] \\
&\text{(According to CA)} \\
&= \pi_{a_1}\mu_{s(a_1,a_1)} + \sum_g (1-\pi_{a_1})\Pr(G_i=g|A_{1i}=a_1, R_i=0)E[Y_i|A_{1i}=a_1, R_i=0, G_i=g, A_{2i}=a_2].
\end{aligned}
$$

The IPW estimator for the value of DTR $\boldsymbol{d}_j$ in SMART-EXAM is

$$\hat{\mu}_{\boldsymbol{d}_j} = \frac{\sum_{i=1}^N W_i^{\boldsymbol{d}_j} Y_i}{\sum_{i=1}^N W_i^{\boldsymbol{d}_j}},$$

where $W_i^{\boldsymbol{d}_j} = \frac{I(A_{1i}=a_1, A_{2i}={a_1^{R_i}}{a_2}^{1-R_i})}{p_{1,a_1}(p_{2,a_2,i})^{(1-R_i)}} = \frac{I(A_{1i}=a_1, A_{2i}={a_1^{R_i}}{a_2}^{1-R_i})}{p_{1,a_1}\{\sum_g I(G_i=g)(p_{2,a_2|a_1,g})^{(1-R_i)}\}}$, and $p_{2,a_2|a_1,g}$ is the randomization probability for treatment $a_2$ when the initial treatment is $a_1$ and in the g-th group.

By the weak law of large numbers,

$$
\begin{aligned}
&\frac{\sum_{i=1}^{N} W_i^{\boldsymbol{d}_j}}{N} \xrightarrow{p} E[W_i^{\boldsymbol{d}_j}] = E[\frac{I(A_{1i}=a_1, A_{2i}=a_1^{R_i}a_2^{1-R_i})}{p_{1,a_1}\{\sum_g I(G_i=g)(p_{2,a_2|a_1,g})^{(1-R_i)}\}}] \\
&= E[E[\frac{I(A_{1i}=a_1, A_{2i}=a_1^{R_i}a_2^{1-R_i})}{p_{1,a_1}\{\sum_g I(G_i=g)(p_{2,a_2|a_1,g})^{(1-R_i)}\}}|A_{1i}, R_i, G_i, A_{2i}]] \\
&= \sum_g \Pr(A_{1i}=a_1, R_i=1, G_i=g, A_{2i}=a_1)E[\frac{1}{p_{1,a_1}}] \\
&+ \sum_g \Pr(A_{1i}=a_1, R_i=0, G_i=g, A_{2i}=a_1)E[\frac{1}{p_{1,a_1}\{\sum_g I(G_i=g)(p_{2,a_2|a_1,g})^{(1-R_i)}\}}] + 0 \\
&= \sum_g p_{1,a_1}\pi_{a_1}\Pr(G_i=g|A_{1i}=a_1, R_i=1)\Pr(A_{2i}=a_1|a_1, R_i=1, G_i=g)\frac{1}{p_{1,a_1}} \\
&+ \sum_g p_{1,a_1}(1-\pi_{a_1})\Pr(G_i=g|A_{1i}=a_1, R_i=0)p_{2,a_2}(a_1,g)E[\frac{1}{p_{1,a_1}(p_{2,a_2|a_1,g})}] \\
&= \pi_{a_1} + (1-\pi_{a_1}) \\
&= 1.
\end{aligned}
$$

According to the weak law of large numbers and the continuous mapping theorem,

$$
\begin{aligned}
\hat{\mu}_{\boldsymbol{d}_j} &= \frac{\sum_{i=1}^{N} W_i^{\boldsymbol{d}_j} Y_i}{\sum_{i=1}^{N} W_i^{\boldsymbol{d}_j}} = \frac{(\sum_{i=1}^{N} W_i^{\boldsymbol{d}_j} Y_i)/N}{(\sum_{i=1}^{N} W_i^{\boldsymbol{d}_j})/N} \xrightarrow{p} \frac{E[W^{\boldsymbol{d}_j}Y]}{E[W^{\boldsymbol{d}_j}]} \\
&= E[W^{\boldsymbol{d}_j}Y] = E[\frac{I(A_{1i}=a_1, A_{2i}=a_1^{R_i}a_2^{1-R_i})Y_i}{p_{1,a_1}\{\sum_g I(G_i=g)(p_{2,a_2|a_1,g})^{(1-R_i)}\}}] \\
&= E[E[\frac{I(A_{1i}=a_1, A_{2i}=a_1^{R_i}a_2^{1-R_i})Y_i}{p_{1,a_1}\{\sum_g I(G_i=g)(p_{2,a_2|a_1,g})^{(1-R_i)}\}}|A_{1i}, R_i, G_i, A_{2i}]] \\
&= \Pr(A_{1i}=a_1, R_i=1, A_{2i}=a_1)E[\frac{Y_i}{p_{1,a_1}}|A_{1i}=a_1, R_i=1, A_{2i}=a_1] \\
&+ \sum_g \Pr(A_{1i}=a_1, R_i=0, G_i=g, A_{2i}=a_1)E[\frac{Y_i}{p_{1,a_1}(p_{2,a_2|a_1,g})}|A_{1i}=a_1, R_i=0, G_i=g, A_{2i}=a_2] \\
&= \frac{p_{1,a_1}\pi_{a_1}}{p_{1,a_1}}E[Y_i|A_{1i}=a_1, R_i=1, A_{2i}=a_2] \\
&+ \sum_g \frac{p_{a_1}(1-\pi_{a_1})\Pr(G_i=g|A_{1i}=a_1, R_i=0)(p_{2,a_2|a_1,g})}{p_{a_1}(p_{2,a_2|a_1,g})}E[Y_i|A_{1i}=a_1, R_i=0, G_i=g, A_{2i}=a_2]) \\
&= \pi_{a_1}\mu_{s(a_1,a_1)} + \sum_g (1-\pi_{a_1})\Pr(G_i=g|A_{1i}=a_1, R_i=0)E[Y_i|A_{1i}=a_1, R_i=0, g_i=G, A_{2i}=a_2] \\
&= \mu_{\boldsymbol{d}_j}.
\end{aligned}
$$

□

## Theorem 3

### Asymptotic normality

First, we derive the influence function of $\hat{\mu}_{\boldsymbol{d}_j}$ as follows:

We know that $\hat{\mu}_{\boldsymbol{d}_j}$ satisfies $g(\hat{\mu}_{\boldsymbol{d}_j}) = \frac{1}{N}\sum_{i=1}^{N} W_i^{\boldsymbol{d}_j}(Y_i - \hat{\mu}_{\boldsymbol{d}_j}) = 0$. Expanding it with respect to $\mu_{\boldsymbol{d}_j}$, we can get

$$\frac{1}{N}\sum_{i=1}^{N} W_i^{\boldsymbol{d}_j}(Y_i - \mu_{\boldsymbol{d}_j}) - (\hat{\mu}_{\boldsymbol{d}_j} - \mu_{\boldsymbol{d}_j})\frac{1}{N}\sum_{i=1}^{N} W_i^{\boldsymbol{d}_j} = 0$$

$$\rightarrow \frac{1}{N}\sum_{i=1}^{N} W_i^{\boldsymbol{d}_j}(Y_i - \mu_{\boldsymbol{d}_j}) - (\hat{\mu}_{\boldsymbol{d}_j} - \mu_{\boldsymbol{d}_j})\frac{1}{N}(\sum_{i=1}^{N} W_i^{\boldsymbol{d}_j} - 1) - (\hat{\mu}_{\boldsymbol{d}_j} - \mu_{\boldsymbol{d}_j}) = 0$$

$$\rightarrow \hat{\mu}_{\boldsymbol{d}_j} - \mu_{\boldsymbol{d}_j} = \frac{1}{N}\sum_{i=1}^{N} W_i^{\boldsymbol{d}_j}(Y_i - \mu_{\boldsymbol{d}_j}) - (\hat{\mu}_{\boldsymbol{d}_j} - \mu_{\boldsymbol{d}_j})\frac{1}{N}\{\sum_{i=1}^{N}(W_i^{\boldsymbol{d}_j} - 1)\}$$

$$\rightarrow \sqrt{N}(\hat{\mu}_{\boldsymbol{d}_j} - \mu_{\boldsymbol{d}_j}) = N^{-1/2}\sum_{i=1}^{N} W_i^{\boldsymbol{d}_j}(Y_i - \mu_{\boldsymbol{d}_j}) - (\hat{\mu}_{\boldsymbol{d}_j} - \mu_{\boldsymbol{d}_j})N^{-1/2}\{\sum_{i=1}^{n}(W_i^{\boldsymbol{d}_j} - 1)\}$$

$$\rightarrow \sqrt{N}(\hat{\mu}_{\boldsymbol{d}_j} - \mu_{\boldsymbol{d}_j}) = N^{-1/2}\sum_{i=1}^{N} \psi_i^{\boldsymbol{d}_j} - (\hat{\mu}_{\boldsymbol{d}_j} - \mu_{\boldsymbol{d}_j})N^{-1/2}\{\sum_{i=1}^{N}(W_i^{\boldsymbol{d}_j} - 1)\}.$$

Because $\hat{\mu}_{\boldsymbol{d}_j} \xrightarrow{p} \mu_{\boldsymbol{d}_j}$, $\hat{\mu}_{\boldsymbol{d}_j} - \mu_{\boldsymbol{d}_j}$ is $o_p(1)$. By the central limit theorem, $N^{-1/2}\{\sum_{i=1}^{N}(W_i^{\boldsymbol{d}_j} - 1)\}$ is $o_p(1)$ given that $E[W_i^{\boldsymbol{d}_j}] = 1$. Therefore, the second term $(\hat{\mu}_{\boldsymbol{d}_j} - \mu_{\boldsymbol{d}_j})N^{-1/2}(\sum_{i=1}^{N} W_i^{\boldsymbol{d}_j} - 1)$ is $o_p(1)$. According to Hampel (1974) and the central limit theorem, we can get

$$\sqrt{N}(\hat{\mu}_{\boldsymbol{d}_j} - \mu_{\boldsymbol{d}_j}) \xrightarrow{d} N(0, \sigma^2_{\boldsymbol{d}_j}),$$

where $\sigma^2_{\boldsymbol{d}_j} = Var(\psi_i^{\boldsymbol{d}_j}) = E[(\psi_i^{\boldsymbol{d}_j})^2]$.

### Derivations for variance and covariance of DTR means

According to the variance formula mentioned above,

$$\sigma^2_{\boldsymbol{d}_j} = Var(\psi_i^{\boldsymbol{d}_j}) = E[(\psi_i^{\boldsymbol{d}_j})^2] = E[(W_i^{\boldsymbol{d}_j})^2(Y_i - \mu_{\boldsymbol{d}_j})^2].$$

We know that $W_i^{\boldsymbol{d}_j} = \frac{I(A_{1i}=a_1, A_{2i}=a_1^{R_i}a_2^{1-R_i})}{p_{1,a_1}\{\sum_g I(G_i=g)(p_{2,a_2|a_1,g})^{(1-R_i)}\}}$, so

$$(W_i^{\boldsymbol{d}_j})^2 = \frac{I(A_{1i} = a_1, A_{2i} = a_1^{R_i}a_2^{1-R_i})}{p^2_{1,a_1}\{\sum_g I(G_i = g)(p^2_{2,a_2|a_1,g})^{(1-R_i)}\}}.$$

The variance of the DTR mean estimator is derived as follows:

$$
\begin{aligned}
\sigma^2_{\boldsymbol{d}_j} &= E[(W_i^{\boldsymbol{d}_j})^2(Y_i-\mu_{\boldsymbol{d}_j})^2] \\
&= E[\frac{I(A_{1i}=a_1, A_{2i}=a_1^{R_i}a_2^{1-R_i})}{p^2_{1,a_1}\{\sum_g I(G_i=g)(p^2_{2,a_2|a_1,g})^{(1-R_i)}\}}(Y_i-\mu_{\boldsymbol{d}_j})^2] \\
&= E[E[\frac{I(A_{1i}=a_1, A_{2i}=a_1^{R_i}a_2^{1-R_i})}{p^2_{1,a_1}\{\sum_g I(G_i=g)(p^2_{2,a_2|a_1,g})^{(1-R_i)}\}}(Y_i-\mu_{\boldsymbol{d}_j})^2|A_{1i},R_i,G_i,A_{2i}]] \\
&= \Pr(A_{1i}=a_1,R_i=1,A_{2i}=a_1)E[\frac{(Y_i-\mu_{\boldsymbol{d}_j})^2}{p^2_{1,a_1}}|A_{1i}=a_1,R_i=1,A_{2i}=a_1] \\
&+\sum_g\left\{\Pr(A_{1i}=a_1,R_i=0,G_i=g,A_{2i}=a_2)\times E[\frac{(Y_i-\mu_{\boldsymbol{d}_j})^2}{p^2_{1,a_1}(p^2_{2,a_2|a_1,g})}|A_{1i}=a_1,R_i=0,G_i=g,A_{2i}=a_2]\right\} \\
&= \frac{p_{1,a_1}\pi_{a_1}}{p^2_{1,a_1}}\times(E[Y_i^2|A_{1i}=a_1,R_i=1,A_{2i}=a_1]+\mu^2_{\boldsymbol{d}_j}-2\mu_{\boldsymbol{d}_j}E[Y_i|A_{1i}=a_1,R_i=1,A_{2i}=a_1]) \\
&+\sum_g\frac{p_{1,a_1}(1-\pi_{a_1})\Pr(G_i=g|A_{1i}=a_1,R_i=0)p_{2,a_2|a_2,g}}{p^2_{1,a_1}(p^2_{2,a_2|a_1,g})} \\
&\times E[Y_i^2|A_{1i}=a_1,R_i=0,G_i=g,A_{2i}=a_2]+\mu^2_{\boldsymbol{d}_j}-2\mu_{\boldsymbol{d}_j}E[Y_i|A_{1i}=a_1,R_i=0,G_i=g,A_{2i}=a_2] \\
&= \frac{\pi_{a_1}}{p_{1,a_1}}(\mu^2_{s(a_1,0)}+\sigma^2_{s(a_1,0)}+\mu^2_{\boldsymbol{d}_j}-2\mu_{\boldsymbol{d}_j}\mu_{s(a_1,0)}) \\
&+\sum_g\left\{\frac{(1-\pi_{a_1})\Pr(G_i=g|A_{1i}=a_1,R_i=0)}{p_{1,a_1}(p_{2,a_2|a_1,g})}(\mu^2_{s(a_1,g,a_2)}+\sigma^2_{s(a_1,g,a_2)}+\mu^2_{\boldsymbol{d}_j}-2\mu_{\boldsymbol{d}_j}\mu_{s(a_1,g,a_2)})\right\} \\
&= \frac{\pi_{a_1}}{p_{1,a_1}}\left\{(\mu_{s(a_1,0)}-\mu_{\boldsymbol{d}_j})^2+\sigma^2_{s(a_1,0)}\right\} \\
&+\sum_g\left\{\frac{(1-\pi_{a_1})\Pr(G_i=g|A_{1i}=a_1,R_i=0)}{p_{1,a_1}(p_{2,a_2|a_1,g})}\{(\mu_{s(a_1,g,a_2)}-\mu_{\boldsymbol{d}_j})^2+\sigma^2_{s(a_1,g,a_2)}\}\right\},
\end{aligned}
$$

where $\mu_{s(a_1,g,a_2)}=E[Y_i|A_{1i}=a_1,R_i=0,G_i=g,A_{2i}=a_2]$, $\sigma^2_{s(a_1,g,a_2)}=\mathrm{Var}(Y_i|A_{1i}=a_1,R_i=0,G_i=g,A_{2i}=a_2)$, $\mu_{a_1,0}=E[Y_i|A_{1i}=a_1,R_i=1]$, $\sigma^2_{s(a_1,0)}=\mathrm{Var}(Y_i|A_{1i}=a_1,R_i=0,G_i=g)$.

So,

$$
\begin{aligned}
\mathrm{Var}(\mu_{\boldsymbol{d}_j}) &= \sigma^2_{\boldsymbol{d}_j}/N \\
&= 1/N(\frac{\pi_{a_1}}{p_{1,a_1}}\{\sigma^2_{s(a_1,0)}+(\mu_{\boldsymbol{d}_j}-\mu_{s(a_1,0)})^2\} \\
&+\sum_g\left\{\frac{(1-\pi_{a_1})\Pr(G=g|A_1=a_1,R=0)}{p_{1,a_1}(p_{2,a_2|a_1,g})}\}\{\sigma^2_{s(a_1,g,a_2)}+(\mu_{\boldsymbol{d}_j}-\mu_{s(a_1,g,a_2)})^2\}\right\}.
\end{aligned}
$$

The covariance of the outcome means for the DTRs that share with the same initial treatment.

i.e., $\mu_{\boldsymbol{d}_j} = \mu_{a_1,a_2}$ and $\mu_{\boldsymbol{d}'_j} = \mu_{a_1,a'_2}$, can be derived by

$$
\begin{aligned}
\sigma_{\boldsymbol{d}_j,\boldsymbol{d}'_j} &= \mathrm{Cov}(\psi_{\boldsymbol{d}_j}, \psi_{\boldsymbol{d}'_j}) = \mathrm{Cov}(W_i^{\boldsymbol{d}_j}(Y_i - \mu_{\boldsymbol{d}_j}), W_i^{\boldsymbol{d}'_j}(Y_i - \mu_{\boldsymbol{d}'_j})) \\
&= E[W_i^{\boldsymbol{d}_j} W_i^{\boldsymbol{d}'_j}(Y_i - \mu_{\boldsymbol{d}_j})(Y_i - \mu_{\boldsymbol{d}'_j})] \\
&= E[\frac{I(A_{1i} = a_1, A_{2i} = a_1^{R_i} a_2^{1-R_i}) I(A_{1i} = a_1, A_{2i} = a_1^{R_i}(a'_2)^{1-R_i})(Y_i - \mu_{\boldsymbol{d}_j})(Y_i - \mu_{\boldsymbol{d}'_j})}{p_{1,a_1}^2 \{\sum_g I(G_i = g)(p_{2,a_2|a_1,g}^2)^{(1-R_i)}\}\{\sum_g I(G_i = g)(p_{2,a_2|a_1,g}^2)^{(1-R_i)}\}}] \\
&= E[E[\frac{I(A_{1i} = a_1, A_{2i} = a_1^{R_i} a_2^{1-R_i}) I(A_{1i} = a_1, A_{2i} = a_1^{R_i}(a'_2)^{1-R_i})(Y_i - \mu_{\boldsymbol{d}_j})(Y_i - \mu_{\boldsymbol{d}'_j})}{p_{1,a_1}^2 \{\sum_g I(G_i = g)(p_{2,a_2|a_1,g}^2)^{(1-R_i)}\}\{\sum_g I(G_i = g)(p_{2,a_2|a_1,g}^2)^{(1-R_i)}\}} | A_{1i}, R_i, G_i, A_{2i}]] \\
&= P(A_{1i} = a_1, R_i = 1, A_{2i} = a_1) E[\frac{(Y_i - \mu_{\boldsymbol{d}_j})(Y_i - \mu_{\boldsymbol{d}'_j})}{p_{1,a_1}^2} | A_{1i} = a_1, R_i = 1, A_{2i} = 0] \\
&= \frac{p_{1,a_1}\pi_{a_1}}{p_{1,a_1}^2}(E[Y_i^2 | A_{1i} = a_1, R_i = 1, A_{2i} = a_1] + \mu_{\boldsymbol{d}_j}\mu_{\boldsymbol{d}'_j} - \mu_{\boldsymbol{d}_j} E[Y_i | A_{1i} = a_1, R_i = 1, A_{2i} = 0] \\
&- \mu_{\boldsymbol{d}'_j} E[Y_i | A_{1i} = a_1, R_i = 1, A_{2i} = 0]) \\
&= \frac{\pi_{a_1}}{p_{1,a_1}}(\sigma_{s(a_1,a_1)}^2 + \mu_{s(a_1,a_1)}^2 + \mu_{\boldsymbol{d}_j}\mu_{\boldsymbol{d}'_j} - \mu_{\boldsymbol{d}_j}\mu_{s(a_1,a_1)} - \mu_{\boldsymbol{d}'_j}\mu_{s(a_1,a_1)}) \\
&= \frac{\pi_{a_1}}{p_{1,a_1}} \left\{ \sigma_{s(a_1,a_1)}^2 + (\mu_{s(a_1,a_1)} - \mu_{\boldsymbol{d}_j})(\mu_{s(a_1,a_1)} - \mu_{\boldsymbol{d}'_j}) \right\}.
\end{aligned}
$$

So,

$$
\begin{aligned}
\mathrm{Cov}(\mu_{\boldsymbol{d}_j}, \mu_{\boldsymbol{d}'_j}) &= \sigma_{\boldsymbol{d}_j,\boldsymbol{d}'_j}/N \\
&= \frac{1}{N} \times \frac{\pi_{a_1}}{p_{1,a_1}} \left\{ \sigma_{s(a_1,a_1)}^2 + (\mu_{s(a_1,a_1)} - \mu_{\boldsymbol{d}_j})(\mu_{s(a_1,a_1)} - \mu_{\boldsymbol{d}'_j}) \right\}.
\end{aligned}
$$

# Web Appendix D: Tables and figures

Web Figure 1: Simulation results for the setting with lower interaction effects in the outcome model, $\eta = -1$, and $\epsilon = 0.2$. The left (right) panel corresponds to the negative ( positive) relationship between preferences and treatment effects. The panels “N=200”, “N=300”, and “N=400” correspond to the scenarios with sample size $N = 200$, $N = 300$, and $N = 400$, respectively; A: the Monte Carlo Mean of the true value of the estimated optimal DTR represented by $E[\mu_{\hat{\boldsymbol{d}}^*}]$; B: the Monte Carlo Mean of the probability of being assigned to the preferred treatment represented by $E[\bar{u}]$; and C: the Monte Carlo Mean of the mean outcome represented by $E[\bar{Y}]$.

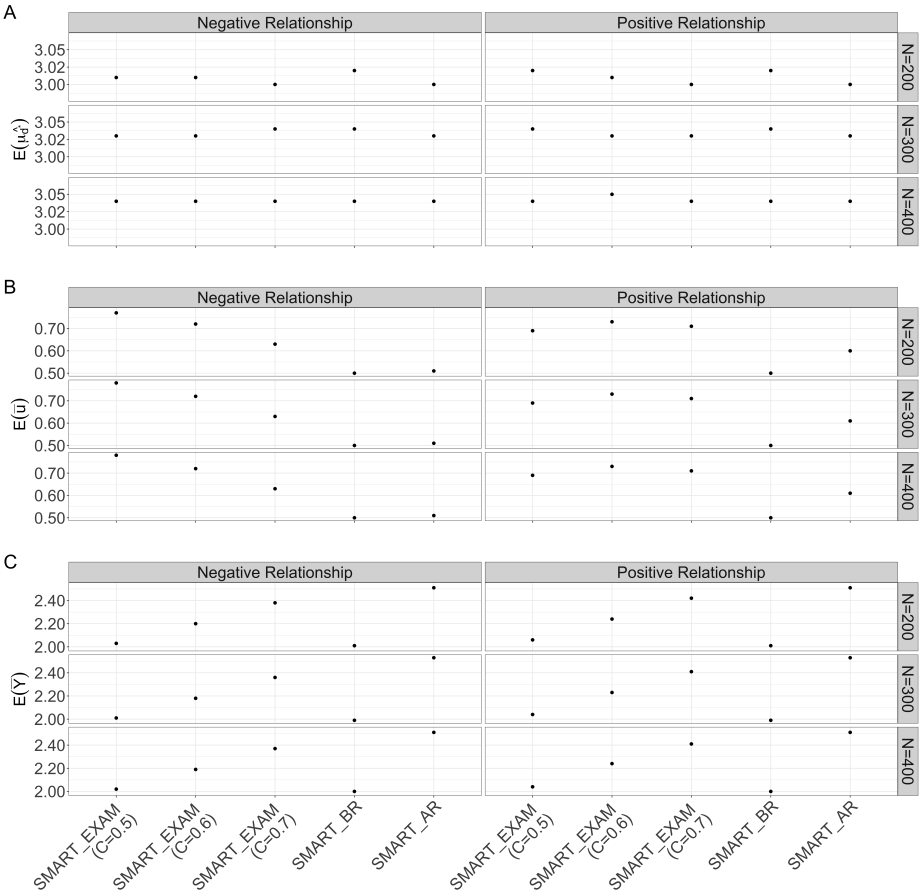

Web Figure 2: Simulation results for settings with different values of $\epsilon$; $\eta = -1$, sample size $N = 200$. The left column corresponds to the Monte Carlo Mean of the true value of the estimated optimal DTR represented by $E[\mu_{\hat{\boldsymbol{d}}^*}]$; the middle column corresponds to the Monte Carlo Mean of the probability of being assigned to the preferred treatment represented by $E[\bar{u}]$; and the right column corresponds to the Monte Carlo Mean of the mean outcome represented by $E[\bar{Y}]$. A: $\epsilon = 0.1$; B: $\epsilon = 0.2$; and C: $\epsilon = 0.3$.

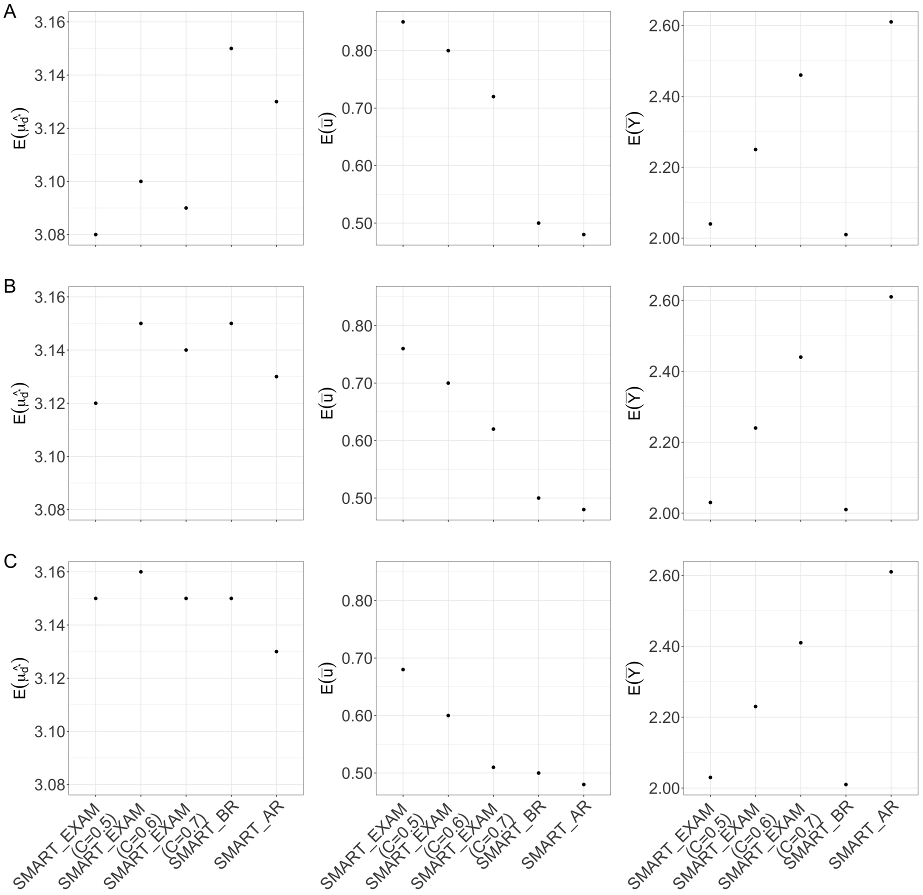

Web Figure 3: Simulation results for settings with different values of $\eta$; $\epsilon = 0.2$, sample size $N = 200$. The left column corresponds to the Monte Carlo Mean of the true value of the estimated optimal DTR represented by $E[\mu_{\hat{\boldsymbol{d}}^*}]$; the middle column corresponds to the Monte Carlo Mean of the probability of being assigned to the preferred treatment represented by $E[\bar{u}]$; and the right column corresponds to the Monte Carlo Mean of the mean outcome represented by $E[\bar{Y}]$. A: $\eta = -0.1$; B: $\eta = -0.5$; and C: $\eta = -1$.

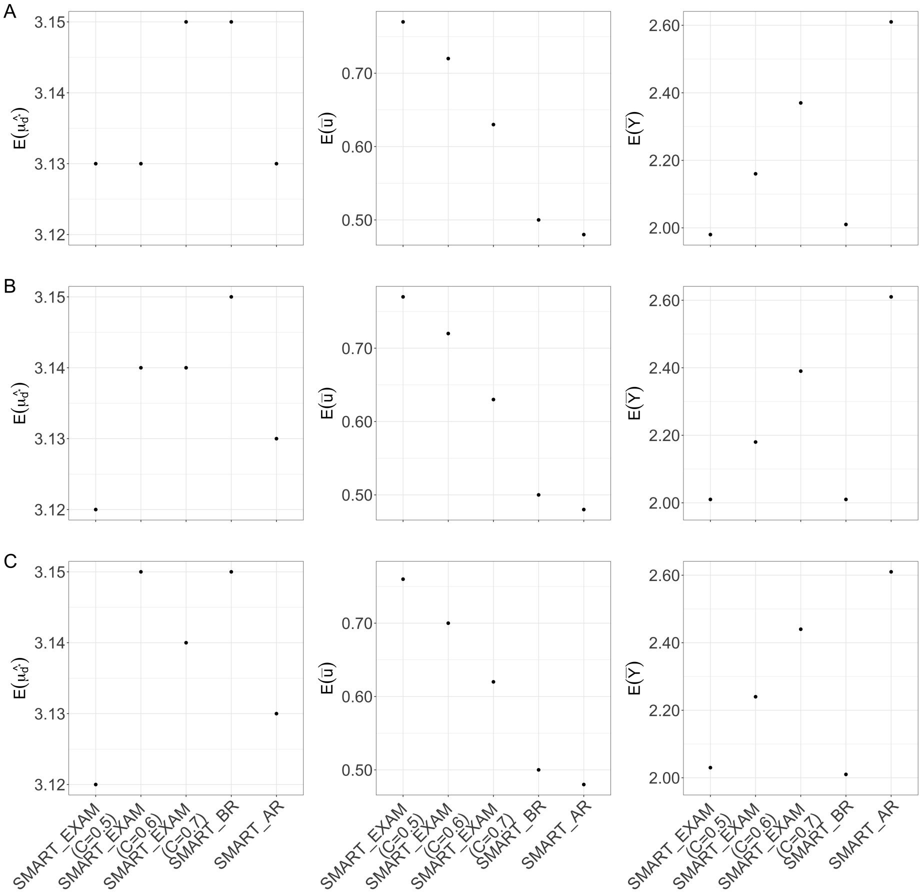

Web Table 1: The operating characteristics of each SMART design when the outcome model has a higher interaction effect and the total sample size is $N = 300$. $\mu_{\boldsymbol{d}_j}$ denotes the true value of the corresponding DTR; $E[\hat{\mu}_{\boldsymbol{d}_j}]$ denotes the Monte Carlo mean of the estimated DTR mean; se$(\hat{\mu}_{\boldsymbol{d}_j})$ denotes the empirical standard error of the estimated DTR mean; $\bar{N}_{\boldsymbol{d}_j}$ is the Monte Carlo mean of the number of participants in the corresponding DTR; se$(N_{\boldsymbol{d}_j})$ denotes the empirical standard error of the number of participants in the corresponding DTR.

| DTR | | SMART-EXAM (C=0.5), Negative | | | | | SMART-EXAM (C=0.5), Positive | | | | |
|---|---|---|---|---|---|---|---|---|---|---|---|
| DTR | $\mu_{\boldsymbol{d}_j}$ | $E[\hat{\mu}_{\boldsymbol{d}_j}]$ | se$(\hat{\mu}_{\boldsymbol{d}_j})$ | $\bar{N}_{\boldsymbol{d}_j}$ | se$(N_{\boldsymbol{d}_j})$ | Pr$(\boldsymbol{d}_j = \hat{\boldsymbol{d}}^*)$ | $E[\hat{\mu}_{\boldsymbol{d}_j}]$ | se$(\hat{\mu}_{\boldsymbol{d}_j})$ | $\bar{N}_{\boldsymbol{d}_j}$ | se$(N_{\boldsymbol{d}_j})$ | Pr$(\boldsymbol{d}_j = \hat{\boldsymbol{d}}^*)$ |
| (-1, -1) | 2.23 | 2.25 | 0.36 | 111.78 | 4.91 | 0.01 | 2.26 | 0.35 | 111.56 | 4.91 | 0.01 |
| (-1, 1) | 2.76 | 2.73 | 0.35 | 113.42 | 4.82 | 0.14 | 2.73 | 0.34 | 113.65 | 4.62 | 0.13 |
| (1, -1) | 1.76 | 1.76 | 0.45 | 111.45 | 4.64 | 0.00 | 1.76 | 0.45 | 111.15 | 4.85 | 0.00 |
| (1, 1) | 3.25 | 3.26 | 0.36 | 113.38 | 4.71 | 0.85 | 3.26 | 0.36 | 113.69 | 4.79 | 0.86 |
| DTR | | SMART-EXAM (C=0.6), Negative | | | | | SMART-EXAM (C=0.6), Positive | | | | |
| DTR | $\mu_{\boldsymbol{d}_j}$ | $E[\hat{\mu}_{\boldsymbol{d}_j}]$ | se$(\hat{\mu}_{\boldsymbol{d}_j})$ | $\bar{N}_{\boldsymbol{d}_j}$ | se$(N_{\boldsymbol{d}_j})$ | Pr$(\boldsymbol{d}_j = \hat{\boldsymbol{d}}^*)$ | $E[\hat{\mu}_{\boldsymbol{d}_j}]$ | se$(\hat{\mu}_{\boldsymbol{d}_j})$ | $\bar{N}_{\boldsymbol{d}_j}$ | se$(N_{\boldsymbol{d}_j})$ | Pr$(\boldsymbol{d}_j = \hat{\boldsymbol{d}}^*)$ |
| (-1, -1) | 2.23 | 2.25 | 0.38 | 105.52 | 5.40 | 0.01 | 2.26 | 0.38 | 104.44 | 5.46 | 0.01 |
| (-1, 1) | 2.76 | 2.74 | 0.31 | 119.68 | 4.58 | 0.12 | 2.73 | 0.30 | 120.76 | 4.25 | 0.11 |
| (1, -1) | 1.76 | 1.76 | 0.47 | 103.75 | 5.30 | 0.00 | 1.76 | 0.49 | 103.65 | 5.42 | 0.00 |
| (1, 1) | 3.25 | 3.25 | 0.32 | 121.08 | 4.60 | 0.87 | 3.26 | 0.32 | 121.19 | 4.51 | 0.88 |
| DTR | | SMART-EXAM (C=0.7), Negative | | | | | SMART-EXAM (C=0.7), Positive | | | | |
| DTR | $\mu_{\boldsymbol{d}_j}$ | $E[\hat{\mu}_{\boldsymbol{d}_j}]$ | se$(\hat{\mu}_{\boldsymbol{d}_j})$ | $\bar{N}_{\boldsymbol{d}_j}$ | se$(N_{\boldsymbol{d}_j})$ | Pr$(\boldsymbol{d}_j = \hat{\boldsymbol{d}}^*)$ | $E[\hat{\mu}_{\boldsymbol{d}_j}]$ | se$(\hat{\mu}_{\boldsymbol{d}_j})$ | $\bar{N}_{\boldsymbol{d}_j}$ | se$(N_{\boldsymbol{d}_j})$ | Pr$(\boldsymbol{d}_j = \hat{\boldsymbol{d}}^*)$ |
| (-1, -1) | 2.23 | 2.25 | 0.40 | 98.99 | 5.80 | 0.02 | 2.25 | 0.40 | 98.26 | 5.96 | 0.01 |
| (-1, 1) | 2.76 | 2.75 | 0.29 | 126.21 | 4.29 | 0.10 | 2.74 | 0.29 | 126.94 | 4.22 | 0.10 |
| (1, -1) | 1.76 | 1.77 | 0.50 | 97.04 | 5.63 | 0.00 | 1.77 | 0.52 | 96.38 | 5.70 | 0.00 |
| (1, 1) | 3.25 | 3.24 | 0.29 | 127.80 | 4.41 | 0.88 | 3.25 | 0.29 | 128.46 | 4.27 | 0.88 |
| DTR | | SMART-BR, Negative | | | | | SMART-BR, Positive | | | | |
| DTR | $\mu_{\boldsymbol{d}_j}$ | $E[\hat{\mu}_{\boldsymbol{d}_j}]$ | se$(\hat{\mu}_{\boldsymbol{d}_j})$ | $\bar{N}_{\boldsymbol{d}_j}$ | se$(N_{\boldsymbol{d}_j})$ | Pr$(\boldsymbol{d}_j = \hat{\boldsymbol{d}}^*)$ | $E[\hat{\mu}_{\boldsymbol{d}_j}]$ | se$(\hat{\mu}_{\boldsymbol{d}_j})$ | $\bar{N}_{\boldsymbol{d}_j}$ | se$(N_{\boldsymbol{d}_j})$ | Pr$(\boldsymbol{d}_j = \hat{\boldsymbol{d}}^*)$ |
| (-1, -1) | 2.23 | 2.26 | 0.30 | 112.53 | 5.34 | 0.01 | 2.26 | 0.30 | 112.53 | 5.34 | 0.01 |
| (-1, 1) | 2.76 | 2.74 | 0.31 | 112.67 | 5.50 | 0.12 | 2.74 | 0.31 | 112.67 | 5.50 | 0.12 |
| (1, -1) | 1.76 | 1.75 | 0.38 | 112.43 | 5.49 | 0.00 | 1.75 | 0.38 | 112.43 | 5.49 | 0.00 |
| (1, 1) | 3.25 | 3.25 | 0.32 | 112.41 | 5.10 | 0.87 | 3.25 | 0.32 | 112.41 | 5.10 | 0.87 |
| DTR | | SMART-AR, Negative | | | | | SMART-AR, Positive | | | | |
| DTR | $\mu_{\boldsymbol{d}_j}$ | $E[\hat{\mu}_{\boldsymbol{d}_j}]$ | se$(\hat{\mu}_{\boldsymbol{d}_j})$ | $\bar{N}_{\boldsymbol{d}_j}$ | se$(N_{\boldsymbol{d}_j})$ | Pr$(\boldsymbol{d}_j = \hat{\boldsymbol{d}}^*)$ | $E[\hat{\mu}_{\boldsymbol{d}_j}]$ | se$(\hat{\mu}_{\boldsymbol{d}_j})$ | $\bar{N}_{\boldsymbol{d}_j}$ | se$(N_{\boldsymbol{d}_j})$ | Pr$(\boldsymbol{d}_j = \hat{\boldsymbol{d}}^*)$ |
| (-1, -1) | 2.23 | 2.29 | 0.35 | 106.98 | 5.79 | 0.01 | 2.29 | 0.35 | 106.98 | 5.79 | 0.01 |
| (-1, 1) | 2.76 | 2.75 | 0.33 | 118.22 | 5.28 | 0.11 | 2.75 | 0.33 | 118.22 | 5.28 | 0.11 |
| (1, -1) | 1.76 | 1.76 | 0.52 | 92.76 | 5.80 | 0.00 | 1.76 | 0.52 | 92.76 | 5.80 | 0.00 |
| (1, 1) | 3.25 | 3.26 | 0.28 | 132.08 | 3.86 | 0.87 | 3.26 | 0.28 | 132.08 | 3.86 | 0.87 |

Web Table 2: The operating characteristics of each SMART design when the outcome model has a higher interaction effect and the total sample size is $N = 400$. $\mu_{\boldsymbol{d}_j}$ denotes the true value of the corresponding DTR; $E[\hat{\mu}_{\boldsymbol{d}_j}]$ denotes the Monte Carlo mean of the estimated DTR mean; se($\hat{\mu}_{\boldsymbol{d}_j}$) denotes the empirical standard error of the estimated DTR mean; $\bar{N}_{\boldsymbol{d}_j}$ is the Monte Carlo mean of the number of participants in the corresponding DTR; se($N_{\boldsymbol{d}_j}$) denotes the empirical standard error of the number of participants in the corresponding DTR.

| DTR | | SMART-EXAM (C=0.5), Negative | | | | | SMART-EXAM (C=0.5), Positive | | | | |
|---|---|---|---|---|---|---|---|---|---|---|---|
| DTR | $\mu_{\boldsymbol{d}_j}$ | $E[\hat{\mu}_{\boldsymbol{d}_j}]$ | se($\hat{\mu}_{\boldsymbol{d}_j}$) | $\bar{N}_{\boldsymbol{d}_j}$ | se($N_{\boldsymbol{d}_j}$) | Pr($\boldsymbol{d}_j = \hat{\boldsymbol{d}}^*$) | $E[\hat{\mu}_{\boldsymbol{d}_j}]$ | se($\hat{\mu}_{\boldsymbol{d}_j}$) | $\bar{N}_{\boldsymbol{d}_j}$ | se($N_{\boldsymbol{d}_j}$) | Pr($\boldsymbol{d}_j = \hat{\boldsymbol{d}}^*$) |
| (-1, -1) | 2.23 | 2.25 | 0.31 | 148.51 | 5.44 | 0.00 | 2.26 | 0.31 | 148.59 | 5.76 | 0.00 |
| (-1, 1) | 2.76 | 2.74 | 0.31 | 151.72 | 5.58 | 0.13 | 2.73 | 0.30 | 151.64 | 5.46 | 0.11 |
| (1, -1) | 1.76 | 1.76 | 0.38 | 148.82 | 5.83 | 0.00 | 1.77 | 0.39 | 148.48 | 5.67 | 0.00 |
| (1, 1) | 3.25 | 3.24 | 0.32 | 151.50 | 5.40 | 0.86 | 3.24 | 0.30 | 151.83 | 5.88 | 0.88 |

| DTR | | SMART-EXAM (C=0.6), Negative | | | | | SMART-EXAM (C=0.6), Positive | | | | |
|---|---|---|---|---|---|---|---|---|---|---|---|
| DTR | $\mu_{\boldsymbol{d}_j}$ | $E[\hat{\mu}_{\boldsymbol{d}_j}]$ | se($\hat{\mu}_{\boldsymbol{d}_j}$) | $\bar{N}_{\boldsymbol{d}_j}$ | se($N_{\boldsymbol{d}_j}$) | Pr($\boldsymbol{d}_j = \hat{\boldsymbol{d}}^*$) | $E[\hat{\mu}_{\boldsymbol{d}_j}]$ | se($\hat{\mu}_{\boldsymbol{d}_j}$) | $\bar{N}_{\boldsymbol{d}_j}$ | se($N_{\boldsymbol{d}_j}$) | Pr($\boldsymbol{d}_j = \hat{\boldsymbol{d}}^*$) |
| (-1, -1) | 2.23 | 2.24 | 0.32 | 140.28 | 6.11 | 0.00 | 2.26 | 0.32 | 138.90 | 6.36 | 0.01 |
| (-1, 1) | 2.76 | 2.75 | 0.28 | 159.95 | 5.47 | 0.10 | 2.73 | 0.27 | 161.33 | 5.33 | 0.09 |
| (1, -1) | 1.76 | 1.76 | 0.40 | 138.62 | 6.62 | 0.00 | 1.76 | 0.42 | 138.70 | 6.09 | 0.00 |
| (1, 1) | 3.25 | 3.25 | 0.27 | 161.70 | 5.15 | 0.90 | 3.25 | 0.27 | 161.62 | 5.21 | 0.91 |

| DTR | | SMART-EXAM (C=0.7), Negative | | | | | SMART-EXAM (C=0.7), Positive | | | | |
|---|---|---|---|---|---|---|---|---|---|---|---|
| DTR | $\mu_{\boldsymbol{d}_j}$ | $E[\hat{\mu}_{\boldsymbol{d}_j}]$ | se($\hat{\mu}_{\boldsymbol{d}_j}$) | $\bar{N}_{\boldsymbol{d}_j}$ | se($N_{\boldsymbol{d}_j}$) | Pr($\boldsymbol{d}_j = \hat{\boldsymbol{d}}^*$) | $E[\hat{\mu}_{\boldsymbol{d}_j}]$ | se($\hat{\mu}_{\boldsymbol{d}_j}$) | $\bar{N}_{\boldsymbol{d}_j}$ | se($N_{\boldsymbol{d}_j}$) | Pr($\boldsymbol{d}_j = \hat{\boldsymbol{d}}^*$) |
| (-1, -1) | 2.23 | 2.24 | 0.33 | 131.48 | 6.55 | 0.01 | 2.25 | 0.34 | 130.83 | 6.66 | 0.01 |
| (-1, 1) | 2.76 | 2.75 | 0.25 | 168.75 | 5.10 | 0.07 | 2.74 | 0.25 | 169.40 | 5.25 | 0.07 |
| (1, -1) | 1.76 | 1.77 | 0.42 | 129.71 | 7.11 | 0.00 | 1.75 | 0.44 | 129.22 | 6.84 | 0.00 |
| (1, 1) | 3.25 | 3.25 | 0.25 | 170.61 | 4.98 | 0.92 | 3.25 | 0.25 | 171.10 | 4.80 | 0.92 |

| DTR | | SMART-BR, Negative | | | | | SMART-BR, Positive | | | | |
|---|---|---|---|---|---|---|---|---|---|---|---|
| DTR | $\mu_{\boldsymbol{d}_j}$ | $E[\hat{\mu}_{\boldsymbol{d}_j}]$ | se($\hat{\mu}_{\boldsymbol{d}_j}$) | $\bar{N}_{\boldsymbol{d}_j}$ | se($N_{\boldsymbol{d}_j}$) | Pr($\boldsymbol{d}_j = \hat{\boldsymbol{d}}^*$) | $E[\hat{\mu}_{\boldsymbol{d}_j}]$ | se($\hat{\mu}_{\boldsymbol{d}_j}$) | $\bar{N}_{\boldsymbol{d}_j}$ | se($N_{\boldsymbol{d}_j}$) | Pr($\boldsymbol{d}_j = \hat{\boldsymbol{d}}^*$) |
| (-1, -1) | 2.23 | 2.24 | 0.27 | 150.14 | 6.16 | 0.00 | 2.24 | 0.27 | 150.14 | 6.16 | 0.00 |
| (-1, 1) | 2.76 | 2.75 | 0.28 | 150.09 | 6.19 | 0.10 | 2.75 | 0.28 | 150.09 | 6.19 | 0.10 |
| (1, -1) | 1.76 | 1.76 | 0.34 | 149.96 | 5.93 | 0.00 | 1.76 | 0.34 | 149.96 | 5.93 | 0.00 |
| (1, 1) | 3.25 | 3.25 | 0.28 | 150.36 | 6.16 | 0.90 | 3.25 | 0.28 | 150.36 | 6.16 | 0.90 |

| DTR | | SMART-AR, Negative | | | | | SMART-AR, Positive | | | | |
|---|---|---|---|---|---|---|---|---|---|---|---|
| DTR | $\mu_{\boldsymbol{d}_j}$ | $E[\hat{\mu}_{\boldsymbol{d}_j}]$ | se($\hat{\mu}_{\boldsymbol{d}_j}$) | $\bar{N}_{\boldsymbol{d}_j}$ | se($N_{\boldsymbol{d}_j}$) | Pr($\boldsymbol{d}_j = \hat{\boldsymbol{d}}^*$) | $E[\hat{\mu}_{\boldsymbol{d}_j}]$ | se($\hat{\mu}_{\boldsymbol{d}_j}$) | $\bar{N}_{\boldsymbol{d}_j}$ | se($N_{\boldsymbol{d}_j}$) | Pr($\boldsymbol{d}_j = \hat{\boldsymbol{d}}^*$) |
| (-1, -1) | 2.23 | 2.24 | 0.30 | 142.35 | 6.73 | 0.00 | 2.24 | 0.30 | 142.35 | 6.73 | 0.00 |
| (-1, 1) | 2.76 | 2.75 | 0.27 | 157.87 | 6.12 | 0.09 | 2.75 | 0.27 | 157.87 | 6.12 | 0.09 |
| (1, -1) | 1.76 | 1.78 | 0.46 | 123.67 | 7.21 | 0.00 | 1.78 | 0.46 | 123.67 | 7.21 | 0.00 |
| (1, 1) | 3.25 | 3.24 | 0.24 | 176.65 | 4.68 | 0.91 | 3.24 | 0.24 | 176.65 | 4.68 | 0.91 |

# Web Appendix E: Data generation in Section 5

For the SMART to be conducted, we assume that there is only one decision point to collect the intermediate response data; thus, the time until entering into stage-2 randomization is the same for all the non-responders, i.e., the non-responders have the same value of $O_{21}$. After analyzing the original data by linear regression, the outcome model for the non-responders is specified as

$$\begin{aligned} Y_i = 2.69 - 0.25O_{11,i} - 0.30O_{12,i} + 0.04O_{13,i} + 0.49O_{14,i} + 0.08A_{1i} - 0.09O_{22,i} + 0.86A_{2i} \\ + 0.19A_{1i}A_{2i} - 1.18O_{22,i}A_{2i} + \tau, \quad \tau \sim N(0,1), \end{aligned} \tag{5}$$

and the outcome model for the responders is specified as

$$Y_i = 3.00 - 0.62O_{11,i} - 0.41O_{12,i} - 0.10O_{13,i} + 0.38O_{14,i} + 0.10A_{1i} + \tau, \quad \tau \sim N(0,1). \tag{6}$$

Based on the original data, we assume that, for baseline variables, $O_{11} \sim$ Bernoulli(0.35), $O_{12} \sim N(-0.12, 1)$, $O_{13} \sim$ Bernoulli(0.31) and $O_{14} \sim$ Bernoulli(0.81). The response rates corresponding to the initial treatment $A_1 = 1$ and $A_1 = -1$ are specified as $\pi_1 = 0.31$ and $\pi_{-1} = 0.37$. The tailoring variable $O_{22} \sim$ Bernoulli(0.42) for those assigned to treatment $A_2 = 1$ and $O_{22} \sim$ Bernoulli(0.53) for those assigned to treatment $A_2 = -1$.

## References

Frank R. H. (1974). The influence curve and its role in robust estimation. *Journal of the American Statistical Association* **69**, 383–393.
